# Supplementary material for: Bayesian Optimization of a Lightweight and Accurate Neural Network for Aerodynamic Performance Prediction
Source: arXiv:2503.19479 source file (2025-03-25)
Supplement: Supplementary file 1 [file appendix.tex]

\section*{Appendix}

\begin{definition}
    Let $f$ be an MLP network (the smaller model) whose hidden layer sizes are $n_1,n_2,...n_m$ where $m$ is the total number of layers.
    Let $F$ be another MLP network (the larger model) whose hidden layer sizes are $N_1,N_2,...N_M$ where $M$ is the total number of layers.
    If $M>m$ and, 
    \[
    N_i>
    \begin{cases}
        n_i &,\forall 1 \le i \le m\\
        0 &,\forall m < i \le M,
    \end{cases}
    \]
    we define the model size of $F$ as being larger than that of $f$.
\end{definition}
\begin{theorem}
    For two MLP network $f$ and $F$, if the model size of $F$ is larger than that of $f$, $F$ has at least the same performance as $f$.
\end{theorem}
\begin{proof}
    Each layer of $f$ can be expressed as $\vec{h}_{i+1}=\vec{a}_{i+1}\vec{h}_i+\vec{b}_{i+1}$, where $\vec{h}_i$ is the hidden neurons of the i\textsuperscript{th} layer, $\vec{a}_{i+1}$ is the weight from $\vec{h}_i$ to $\vec{h}_{i+1}$, and $\vec{b}_{i+1}$ is the bias.
    Similarly, those of $F$ is $\vec{H}_{i+1}=\vec{A}_i\vec{H}_i+\vec{B}_i$.
    For the same input $\vec{x}$, it is possible to set $\vec{A}_1=\begin{bmatrix}
        \vec{a}_1 & \vec{0}
    \end{bmatrix}^\top$ and $\vec{B}_1=\begin{bmatrix}
        \vec{b}_1 & \vec{0}
    \end{bmatrix}^\top$ so that
    \[
    \vec{H}_1=\vec{A}_1\vec{x}+\vec{b}_1=
    \begin{bmatrix}
        \vec{a}_1\\
        \vec{0}
    \end{bmatrix}\vec{x}
    +\begin{bmatrix}
        \vec{b}_1\\
        \vec{0}
    \end{bmatrix}=
    \begin{bmatrix}
        \vec{a}_1 \vec{x}+\vec{b}_1\\
        \vec{0}
    \end{bmatrix}=
    \begin{bmatrix}
        \vec{h}_1\\
        \vec{0}
    \end{bmatrix}.
    \]
    For subsequent layers where $1 \le i \le m$, we can construct $\vec{A}_{i+1}=\begin{bmatrix}
        \vec{a}_{i+1} & \vec{0}\\
        \vec{0} & \vec{0}
    \end{bmatrix}$ and $\vec{B}_1=\begin{bmatrix}
        \vec{b}_{i+1} \\
        \vec{0}
    \end{bmatrix}$ so that
    \[
    \vec{H}_{i+1}=\vec{A}_i\vec{H}_i+\vec{B}_i=
    \begin{bmatrix}
        \vec{a}_{i+1} & \vec{0}\\
        \vec{0} & \vec{0}
    \end{bmatrix}
    \begin{bmatrix}
        \vec{h}_i\\
        \vec{0}
    \end{bmatrix}
    +\begin{bmatrix}
        \vec{b}_{i+1}\\
        \vec{0}
    \end{bmatrix}=
    \begin{bmatrix}
        \vec{a}_{i+1} \vec{h}_i+\vec{b}_{i+1}\\
        \vec{0}
    \end{bmatrix}=
    \begin{bmatrix}
        \vec{h}_{i+1}\\
        \vec{0}
    \end{bmatrix}.
    \]
    For additional layers in $F$ but not in $f$, i.e. for $m < i \le M$,  it is trivial to construct $\vec{A}_{i+1}=\begin{bmatrix}
        \vec{I} & \vec{0}\\
        \vec{0} & \vec{0}
    \end{bmatrix}$ and $\vec{B}_{i+1}=\vec{0}$ so that
    \[
    \vec{H}_{i+1}=
    \begin{bmatrix}
        \vec{I} & \vec{0}\\
        \vec{0} & \vec{0}
    \end{bmatrix}
    \begin{bmatrix}
        \vec{h}_m\\
        \vec{0}
    \end{bmatrix}+\vec{0}=
    \begin{bmatrix}
        \vec{h}_m\\
        \vec{0}
    \end{bmatrix}.
    \]
    Finally,
    \[
    \vec{Y}=
    \begin{bmatrix}
        \vec{a}_{m+1} & \vec{0}
    \end{bmatrix}
    \begin{bmatrix}
        \vec{h}_m\\
        \vec{0}
    \end{bmatrix}+
    \begin{bmatrix}
        \vec{b}_{m+1}\\
        \vec{0}
    \end{bmatrix}=\vec{y},
    \]
    where $\vec{Y}=F(\vec{x})$ and $\vec{y}=f(\vec{x})$.
    We have shown that $F$ can be equivalent to $f$, thus having at least the same performance.
\end{proof}
